# Supplementary material for: An extremely low-density and temperate giant exoplanet
Source: arXiv:1911.07355 ancillary file (2019-11-17)
Supplement: Supplementary file 1 [file HIP41378_Supplements_arXiv.pdf]

# An extremely low-density and temperate giant exoplanet

*Supplementary Informations*

A. Santerne[1], L. Malavolta[2], M. R. Kosiarek[3,4], F. Dai[5,6,7], C. D. Dressing[8], X. Dumusque[9], N. C. Hara[9,10], T. A. Lopez[1], A. Mortier[11], A. Vanderburg[12], V. Adibekyan[13], D. J. Armstrong[14,15], D. Barrado[16], S. C. C. Barros[13], D. Bayliss[15], D. Berardo[17], I. Boisse[1], A. S. Bonomo[18], F. Bouchy[9], D. J. A. Brown[14,15], L. A. Buchhave[19], R. P. Butler[20], A. Collier Cameron[21], R. Cosentino[22], J. D. Crane[24], I. J. M. Crossfield[5,23], M. Damasso[18], M. R. Deleuil[1], E. Delgado Mena[13], O. Demangeon[13], R. F. Díaz[25,26], J.-F. Donati[27], P. Figueira[28,13], B. J. Fulton[29], A. Ghedina[22], A. Harutyunyan[22], G. Hébrard[30], L. A. Hirsch[31], S. Hojjatpanah[13,32], A. W. Howard[33], H. Isaacson[8], D. W. Latham[34], J. Lillo-Box[16,28], M. López-Morales[34], C. Lovis[9], A. F. Martinez Fiorenzano[22], E. Molinari[35], O. Mousis[1], C. Moutou[27], C. Nava[34], L. D. Nielsen[9], H. P. Osborn[1], E. A. Petigura[36], D. F. Phillips[34], D. L. Pollacco[14,15], E. Poretti[22], K. Rice[37,38], N. C. Santos.[13,32], D. Ségransan[9], S. A. Shectman[24], E. Sinukoff[33], S. G. Sousa[13], A. Sozzetti[18], J. K. Teske[24,39], S. Udry[9], A. Vigan[1], S. X. Wang[24], C. A. Watson[40], L. M. Weiss[41], P. J. Wheatley[14,15], J. N. Winn[6]

[1]*Aix Marseille Univ, CNRS, CNES, LAM, Marseille, France*
[2]*INAF - Osservatorio Astrofisico di Catania, Via S.Sofia 78, 95123 Catania, Italy*
[3]*Department of Astronomy and Astrophysics, University of California, Santa Cruz, CA 95064, USA*
[4]*NSF Graduate Research Fellow*
[5]*Department of Physics and Kavli Institute for Astrophysics and Space Research, Massachusetts Institute of Technology, Cambridge, MA, 02139, USA*
[6]*Department of Astrophysical Sciences, Princeton University, 4 Ivy Lane, Princeton, NJ 08544 USA*
[7]*Division of Geological and Planetary Sciences, California Institute of Technology,1200 East California Blvd, Pasadena, CA, USA 91125*
[8]*Department of Astronomy, University of California, Berkeley, Berkeley, CA 94720, USA*
[9]*Department of Astronomy of the University of Geneva, 51 Chemin des Maillettes, 1290 Versoix, Switzerland*
[10]*CHEOPS fellow*
[11]*Cavendish Laboratory and Kavli Institute for Cosmology, University of Cambridge, J.J. Thomson Avenue, Cambridge CB3 0HE, UK*
[12]*Department of Astronomy, The University of Texas at Austin, Austin, TX 78712, USA*
[13]*Instituto de Astrofísica e Ciências do Espaçco, Universidade do Porto, CAUP, Rua das Estrelas, 4150-762 Porto, Portugal*
[14]*Centre for Exoplanets and Habitability, University of Warwick, Gibbet Hill Road, Coventry, CV4 7AL, UK*
[15]*Department of Physics, University of Warwick, Gibbet Hill Road, Coventry, CV4 7AL, UK*
[16]*Centro de Astrobiología (CSIC-INTA), ESAC campus 28692 Villanueva de la Cañada (Madrid), Spain*
[17]*Department of Physics, and Kavli Institute for Astrophysics and Space Research, Massachusetts*

*Institute of Technology, Cambridge, MA, USA*
[18]*INAF - Osservatorio Astrofisico di Torino, via Osservatorio 20, 10025 Pino Torinese, Italy*
[19]*DTU Space, National Space Institute, Technical University of Denmark, Elektrovej 328, DK-2800 Kgs. Lyngby, Denmark*
[20]*Department of Terrestrial Magnetism, Carnegie Institution for Science, 5241 Broad Branch Road NW, Washington DC 20015*
[21]*Centre for Exoplanet Science, SUPA School of Physics and Astronomy, University of St Andrews, North Haugh, St Andrews KY16 9SS, UK*
[22]*INAF - Fundacion Galileo Galilei, Rambla Josè Ana Fernandez Pèrez, 7 - Breña Baja, TF - Spain*
[23]*The University of Kansas, Department of Physics and Astronomy, Malott Room 1082, 1251 Wescoe Hall Drive, Lawrence, KS, 66045, USA*
[24]*The Observatories of the Carnegie Institution for Science, 813 Santa Barbara Street, Pasadena, CA, USA 91101*
[25]*Universidad de Buenos Aires, Facultad de Ciencias Exactas y Naturales, Buenos Aires, Argentina*
[26]*CONICET - Universidad de Buenos Aires. Instituto de Astronomía y Física del Espacio (IAFE), Buenos Aires, Argentina*
[27]*IRAP, 14 avenue Edouard Belin 31400 Toulouse, France*
[28]*European Southern Observatory, Alonso de Cordova 3107, Vitacura, Santiago, Chile*
[29]*NASA Exoplanet Science Institute / Caltech-IPAC, Pasadena, CA, USA 91106*
[30]*Institut d'Astrophysique de Paris, UMR7095 CNRS, Université Pierre & Marie Curie, 98bis boulevard Arago, 75014 Paris, France*
[31]*Kavli Institute for Particle Astrophysics and Cosmology, Stanford University, Stanford, CA, USA*
[32]*Departamento de Fisica e Astronomia, Faculdade de Ciências, Universidade do Porto, Rua Campo Alegre, 4169-007 Porto, Portugal*
[33]*California Institute of Technology, Pasadena, CA 91125, USA*
[34]*Center for Astrophysics | Harvard & Smithsonian, 60 Garden Street, Cambridge, MA 02138, USA*
[35]*INAF Osservatorio Astronomico di Cagliari & REM - Via della Scienza 5 - 09047 Selargius CA, Italy*
[36]*Department of Physics & Astronomy, University of California Los Angeles, Los Angeles, CA 90095, USA*
[37]*SUPA, Institute for Astronomy, University of Edinburgh, Royal Observatory, Blackford Hill, Edinburgh, EH93HJ, UK*
[38]*Centre for Exoplanet Science, University of Edinburgh, Edinburgh, UK*
[39]*NASA Hubble Fellow*
[40]*Astrophysics Research Centre, Queen's University Belfast, Belfast BT7 1NN, UK*
[41]*Institute for Astronomy, 2680 Woodlawn Dr., Honolulu, HI 96822, USA*

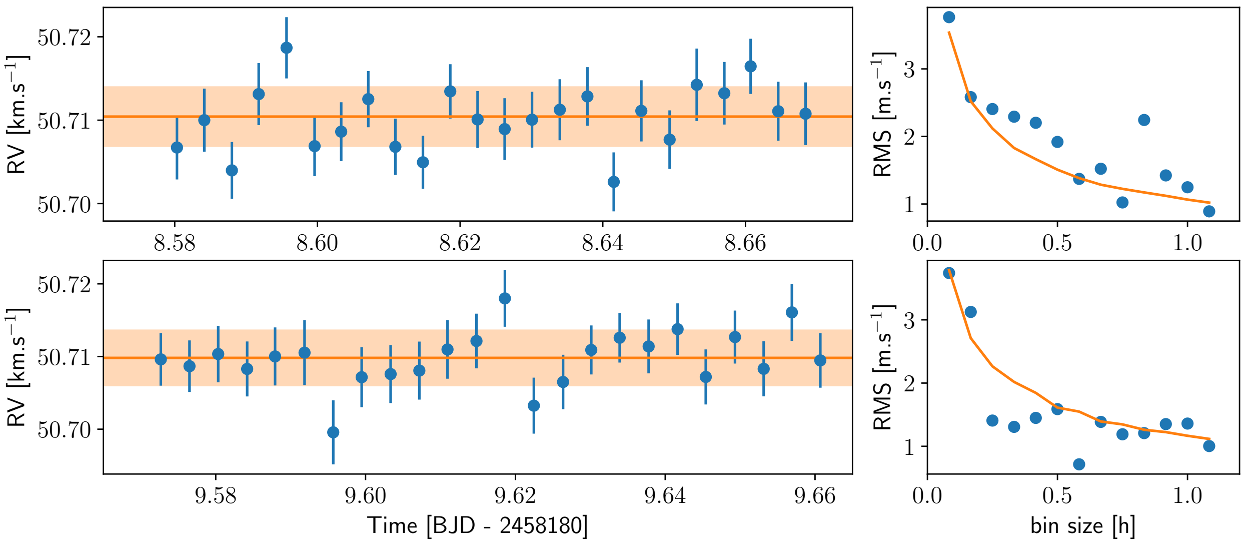


Supplementary Figure 1: **HARPS high-cadence time series.** The left panels display the radial velocities (RV, in blue) over time for the two nights. The horizontal orange line is the median of the data over the night while the orange zone represent the median photon noise reached over the night. The right panels show the RMS of the radial velocities measured in different bins (in blue) and compared to the expected photon noise over the bin (in orange).

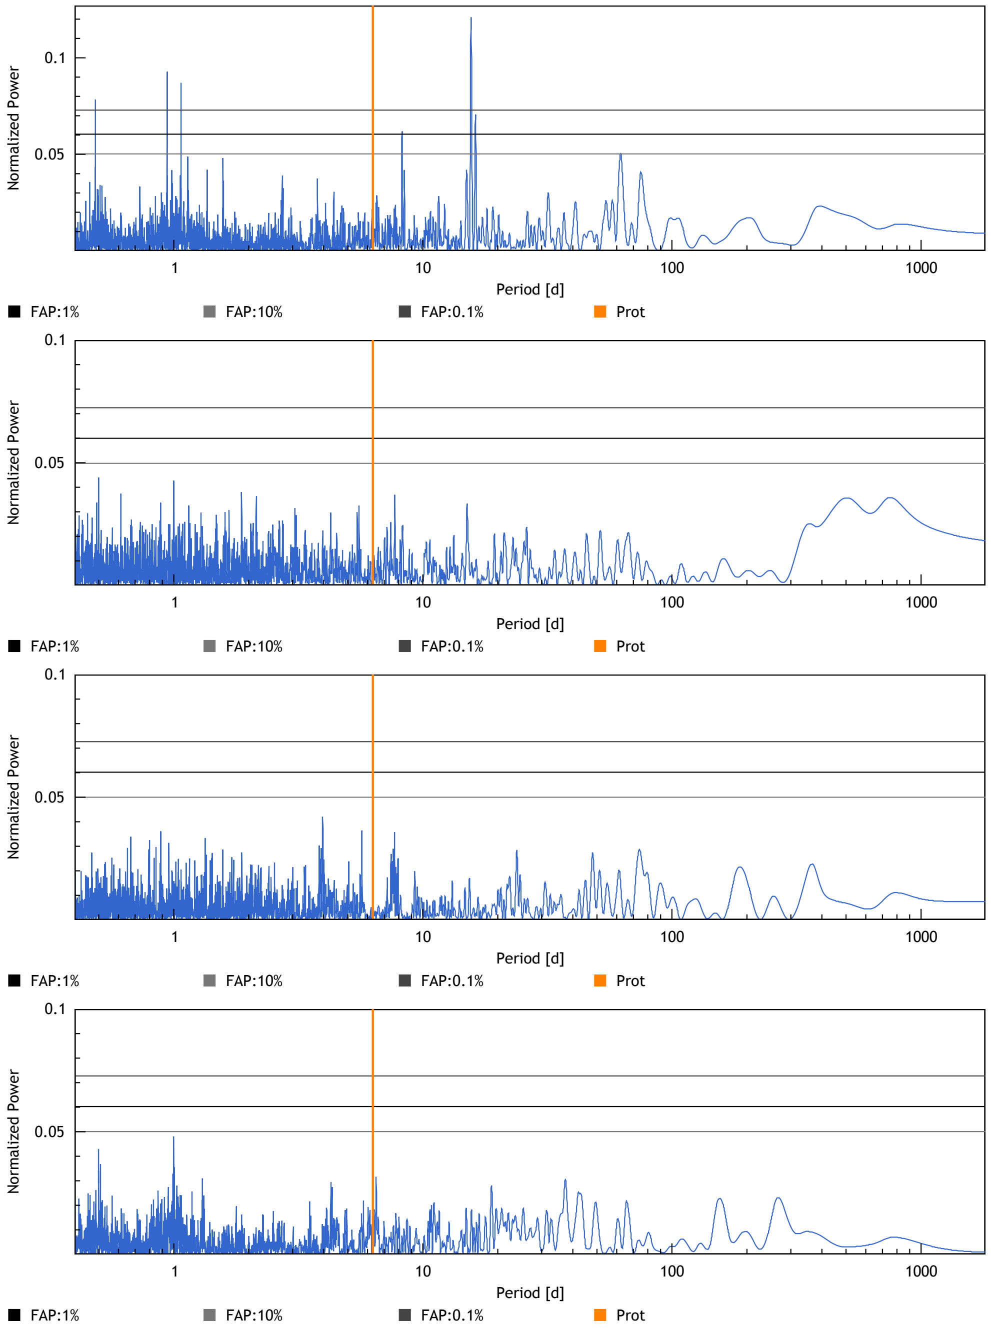


Supplementary Figure 2: **Periodograms of the HIP41378 HARPS and HARPS data.** Generalised Lomb-Scargle periodograms of the RV, FWHM, BIS, and Sindex (from top to bottom) based on the HARPS and HARPS-N nightly-binned data. The false-alarm probabilities at 10%, 1%, and 0.1% are displayed (horizontal lines) together with the rotation period of the star (vertical line).

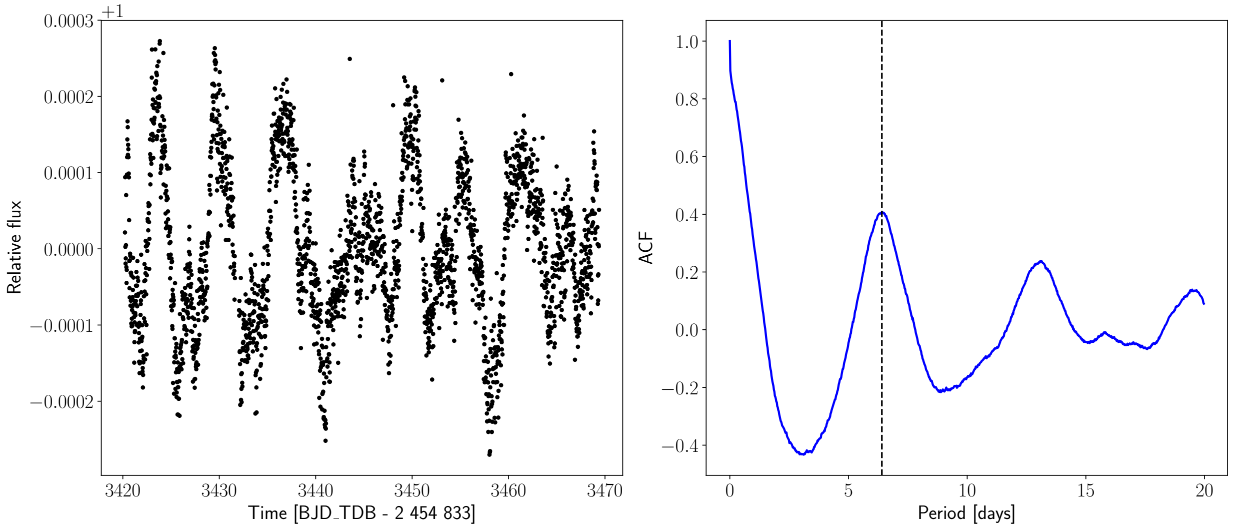


Supplementary Figure 3: **Photometric analysis of the stellar variability.** The left panel shows the $K2$ C18 reduced data corrected for the planetary transit but not flattened. The right panel shows the autocorrelation function of the data displayed in the left panel. The rotation period of the star is indicated by the dashed line.

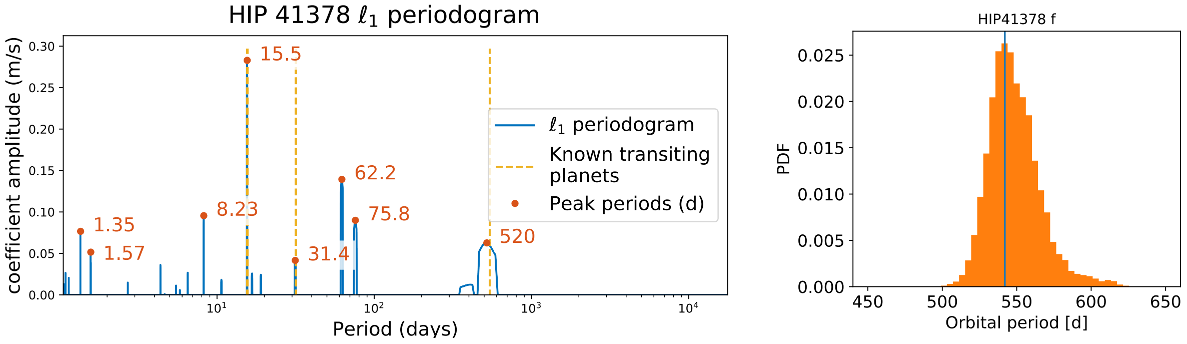


Supplementary Figure 4: **Results of the preliminary analysis of the radial velocities of HIP41378.** The left panel shows the $\ell_1$ periodogram of the data assuming an instrumental white noise of 2m.s$^{-1}$ for both HARPS and HARPS-N and 4m.s$^{-1}$ for both HIRES and PFS. The periods of the main signals are labeled and the periods of the transiting planets $b$, $c$, and $f$ are indicated by the vertical lines. The amplitudes are known to be biased towards lower values. The right panel show the posterior distribution function (PDF) for the orbital period of HIP41378 $f$ marginalised over the other parameters. This PDF results from the MCMC analysis of the radial velocity data assuming a broad prior for the periods of the outer transiting planets. The 542-d orbital-period solution constrained by the $K2$ photometry is indicated by the vertical line and perfectly match with the mode of the PDF.

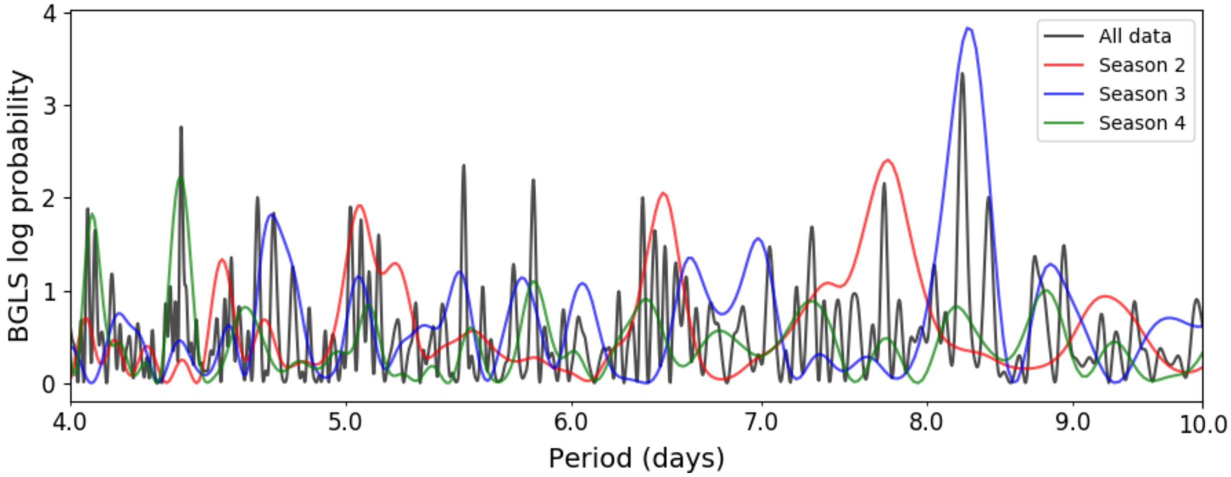


Supplementary Figure 5: **BGLS periodogram of the radial velocity residuals.** The black curve is the periodogram using all data while the red, blue, and green are from the season 2, 3, and 4 (respectively).

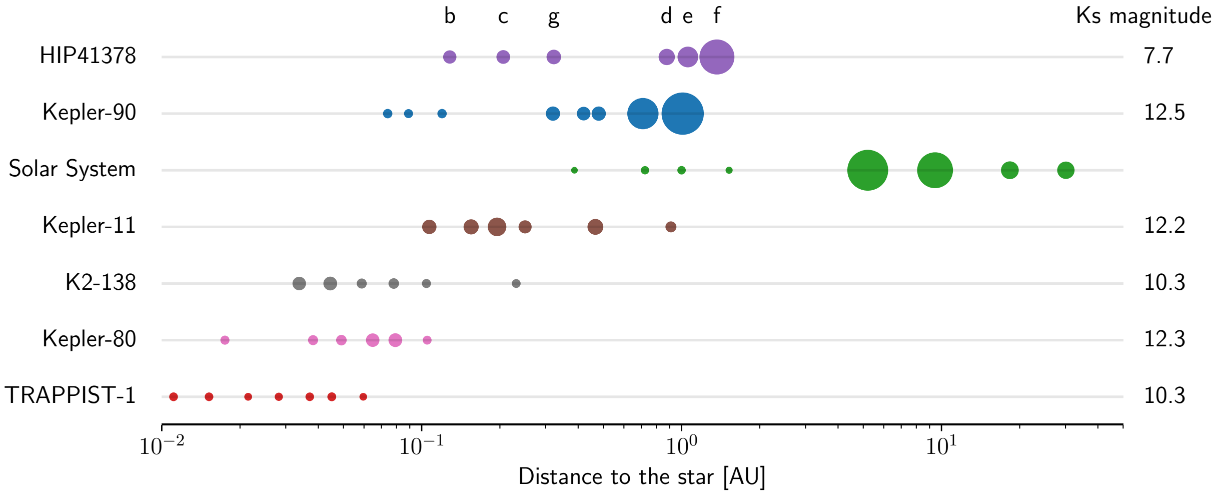


Supplementary Figure 6: **Comparison between HIP41378 and other multi-planetary systems.** The planets of each systems are displayed as function of their distance to the host star. The mark size scales with the radius of the planet. Systems are ranked from bottom to top by increasing $T_{eff}$ of the host star. Only systems with at least 6 planets and detected by transit are displayed here. The magnitude in the Ks-band of the host star is indicated on the right. The solar system is shown for comparison.

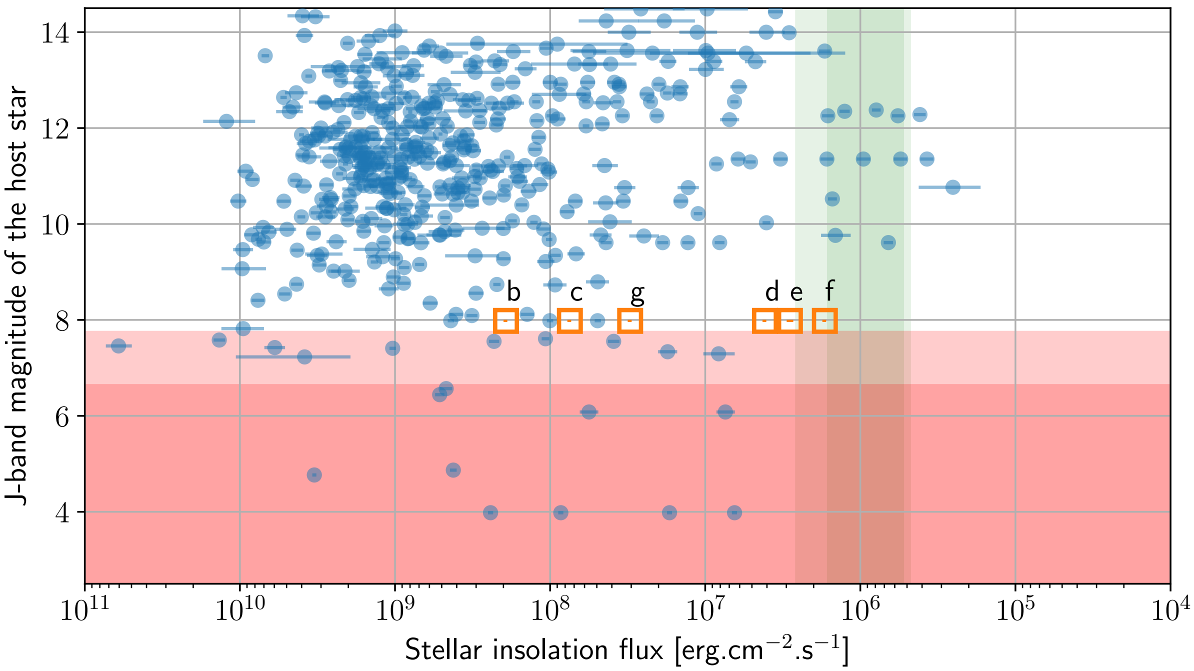


Supplementary Figure 7: **Stellar insolation flux and J-band magnitude of the host star.** The five transiting planets in the HIP41378 system are plotted with the orange rectangles. The green zone represent the conservative (green) and optimistic (light green) habitable zone (Kopparapu et al., 2013). The red zones indicated the (worst case) saturation level for JWST / NIRSpec in medium- (light red) and high-resolution (red) modes. HIP41378 is just right in terms of magnitude to avoid saturation with NIRSpec.

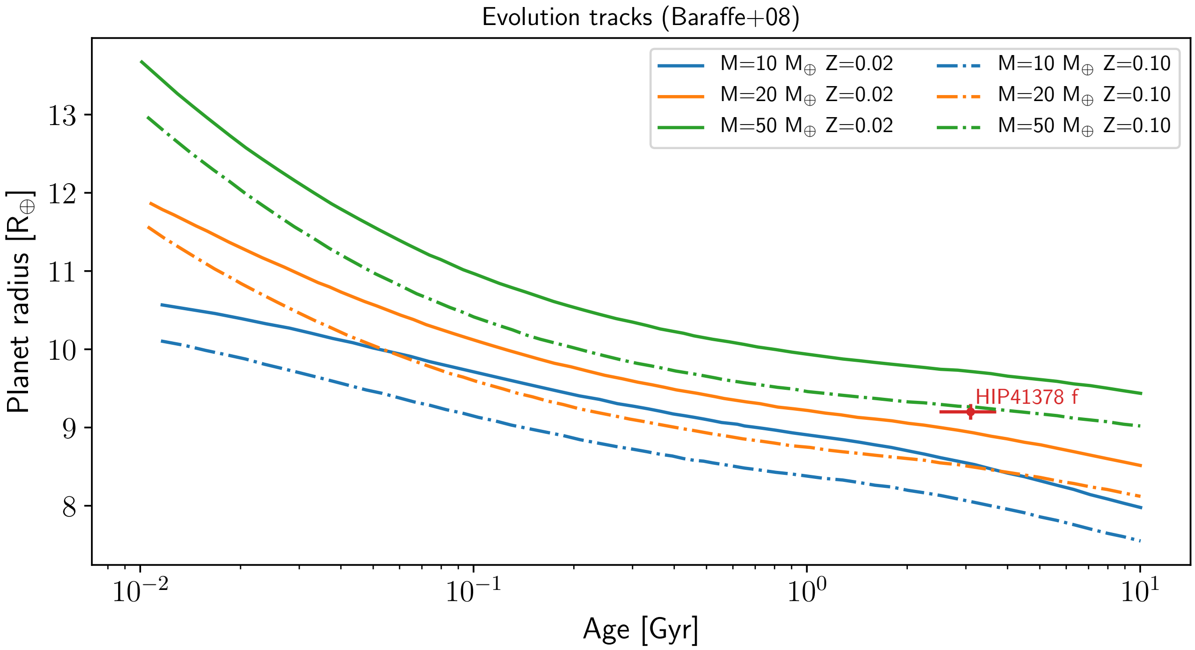


Supplementary Figure 8: **Comparison between HIP41378 f and evolutionary tracks of low-mass exoplanets.** The planetary radius is displayed as function of the system's age. The tracks are from the models of Baraffe et al. (2008) for a 10-$M_\oplus$ (blue), 20-$M_\oplus$ (orange), and 50-$M_\oplus$ (green) planet with different metal mass fraction of Z=0.02 (solid lines), corresponding to a solar value, or Z=0.10 (dot-dashed lines). The 20-$M_\oplus$, and 50-$M_\oplus$ models are displayed for comparison even if they are excluded by the data. The planet HIP41378 $f$ exhibits an abnormally large radius and needs a sub-Solar metallicity to explain it.

Supplementary Table 1: **Spectral energy distribution of the star HIP41378.**

| band | mag | error | Source |
|---|---|---|---|
| Johnson B | 9.516 | 0.022 | TYCHO |
| Johnson V | 8.980 | 0.018 | TYCHO |
| 2MASS J | 7.982 | 0.026 | 2-MASS |
| 2MASS H | 7.786 | 0.038 | 2-MASS |
| 2MASS Ks | 7.722 | 0.031 | 2-MASS |
| WISE 1 | 7.662 | 0.029 | AllWISE |
| WISE 2 | 7.732 | 0.020 | AllWISE |
| WISE 3 | 7.732 | 0.018 | AllWISE |
| WISE 4 | 7.860 | 0.248 | AllWISE |

Supplementary Table 2: **HARPS data.** Nightly-binned radial velocities from the HARPS spectrograph. A calibration noise at the level of 0.5m.s$^{-1}$ was been added to the uncertainties.

| Time [BJD] | RV [km.s$^{-1}$] | $\sigma_{RV}$ [km.s$^{-1}$] |
|---|---|---|
| 2457780.688666 | 50.708585 | 0.001987 |
| 2457781.671453 | 50.706095 | 0.001756 |
| 2457782.673409 | 50.709012 | 0.001745 |
| 2457784.724333 | 50.715344 | 0.001595 |
| 2457785.704812 | 50.718927 | 0.001506 |
| 2457787.701341 | 50.709967 | 0.001514 |
| 2457789.730856 | 50.709713 | 0.001498 |
| 2457790.677303 | 50.715433 | 0.001787 |
| 2457791.740260 | 50.712863 | 0.001389 |
| 2457795.658322 | 50.708390 | 0.001522 |
| 2457796.668201 | 50.712369 | 0.001472 |
| 2457797.659210 | 50.707238 | 0.001438 |
| 2457798.665171 | 50.713145 | 0.001501 |
| 2457799.643897 | 50.717704 | 0.001804 |
| 2457800.556180 | 50.708313 | 0.002669 |
| 2457801.651597 | 50.714471 | 0.001434 |
| 2457802.630778 | 50.710170 | 0.001602 |
| 2457803.609344 | 50.712172 | 0.001457 |
| 2457810.617176 | 50.710441 | 0.001556 |
| 2457811.637072 | 50.707780 | 0.001500 |
| 2457814.649179 | 50.713928 | 0.001409 |
| 2457815.608463 | 50.714792 | 0.001393 |
| 2457817.597421 | 50.713203 | 0.001472 |
| 2457818.560320 | 50.713989 | 0.001447 |

Continued on next page

**Supplementary Table 2 – continued from previous page**

| Time | RV | $\sigma_{RV}$ |
|---|---|---|
| 2457822.616058 | 50.711503 | 0.001512 |
| 2457823.579657 | 50.718199 | 0.001530 |
| 2457824.598187 | 50.708786 | 0.001668 |
| 2457826.555549 | 50.711775 | 0.001796 |
| 2457827.524114 | 50.706771 | 0.002606 |
| 2457831.596747 | 50.715068 | 0.001411 |
| 2457834.591148 | 50.711034 | 0.001573 |
| 2457836.592265 | 50.711347 | 0.001790 |
| 2457837.539322 | 50.712058 | 0.001672 |
| 2458054.860569 | 50.713271 | 0.002046 |
| 2458055.872428 | 50.710614 | 0.001777 |
| 2458056.859389 | 50.704587 | 0.001681 |
| 2458057.874883 | 50.708572 | 0.001709 |
| 2458068.837126 | 50.713865 | 0.002222 |
| 2458069.842369 | 50.718083 | 0.001784 |
| 2458071.835753 | 50.711746 | 0.001519 |
| 2458073.837603 | 50.708924 | 0.001365 |
| 2458074.841128 | 50.710184 | 0.001403 |
| 2458075.841568 | 50.708906 | 0.001486 |
| 2458076.832538 | 50.713775 | 0.001556 |
| 2458077.836976 | 50.712914 | 0.001368 |
| 2458078.832457 | 50.715441 | 0.001314 |
| 2458079.823893 | 50.711936 | 0.000967 |
| 2458081.818027 | 50.714445 | 0.001571 |
| 2458088.836299 | 50.709591 | 0.001609 |
| 2458089.802866 | 50.707718 | 0.001875 |
| 2458090.803635 | 50.706649 | 0.001728 |
| 2458091.816640 | 50.707316 | 0.001626 |
| 2458092.800783 | 50.710098 | 0.001586 |
| 2458107.798720 | 50.708133 | 0.001513 |
| 2458108.798513 | 50.712050 | 0.001586 |
| 2458109.793052 | 50.709332 | 0.001680 |
| 2458110.750088 | 50.712864 | 0.001782 |
| 2458111.803275 | 50.718681 | 0.001311 |
| 2458112.795314 | 50.712667 | 0.001282 |
| 2458113.814094 | 50.712729 | 0.001365 |
| 2458114.787223 | 50.714132 | 0.001258 |
| 2458115.780618 | 50.716018 | 0.001348 |
| 2458116.775995 | 50.713647 | 0.001458 |
| 2458117.779640 | 50.711352 | 0.001374 |

Continued on next page

**Supplementary Table 2 – continued from previous page**

| Time | RV | $\sigma_{RV}$ |
|---|---|---|
| 2458118.778799 | 50.710820 | 0.001299 |
| 2458123.761513 | 50.712690 | 0.001329 |
| 2458124.854217 | 50.713795 | 0.001751 |
| 2458125.749197 | 50.714901 | 0.001520 |
| 2458126.751302 | 50.718077 | 0.001704 |
| 2458127.755449 | 50.717583 | 0.001912 |
| 2458129.707020 | 50.717747 | 0.002070 |
| 2458130.707116 | 50.717528 | 0.002208 |
| 2458132.697083 | 50.716473 | 0.001896 |
| 2458149.668360 | 50.713333 | 0.002207 |
| 2458156.713083 | 50.705036 | 0.001879 |
| 2458158.668657 | 50.714031 | 0.001277 |
| 2458159.665704 | 50.714812 | 0.001533 |
| 2458160.665177 | 50.717502 | 0.001671 |
| 2458161.692582 | 50.711872 | 0.001452 |
| 2458162.661157 | 50.711455 | 0.001507 |
| 2458188.624123 | 50.710107 | 0.000909 |
| 2458189.617815 | 50.709838 | 0.000957 |
| 2458190.545680 | 50.713492 | 0.001637 |
| 2458198.572369 | 50.711311 | 0.001038 |
| 2458199.580816 | 50.709512 | 0.001053 |
| 2458200.516540 | 50.711366 | 0.001055 |
| 2458201.548224 | 50.713742 | 0.001149 |
| 2458202.564756 | 50.712933 | 0.001209 |
| 2458203.532729 | 50.714947 | 0.001020 |
| 2458204.536623 | 50.715267 | 0.001011 |
| 2458401.876758 | 50.715019 | 0.002773 |
| 2458404.877514 | 50.700895 | 0.002631 |
| 2458406.893517 | 50.702322 | 0.002952 |
| 2458407.895430 | 50.706174 | 0.002093 |
| 2458409.871789 | 50.707213 | 0.002178 |
| 2458410.873287 | 50.713278 | 0.002043 |
| 2458411.879635 | 50.708349 | 0.002052 |
| 2458412.877510 | 50.717917 | 0.002040 |
| 2458413.875050 | 50.709202 | 0.001906 |
| 2458414.874418 | 50.713945 | 0.002104 |
| 2458415.869886 | 50.709461 | 0.002164 |
| 2458416.876328 | 50.707744 | 0.002012 |
| 2458417.873197 | 50.708380 | 0.002758 |
| 2458418.877729 | 50.709098 | 0.001816 |

Continued on next page

**Supplementary Table 2 – continued from previous page**

| Time | RV | $\sigma_{RV}$ |
|---|---|---|
| 2458419.875108 | 50.709422 | 0.002019 |
| 2458422.873298 | 50.709914 | 0.003003 |
| 2458423.872470 | 50.713808 | 0.001792 |
| 2458424.878611 | 50.712277 | 0.002219 |
| 2458425.876013 | 50.710530 | 0.001754 |
| 2458426.874746 | 50.713143 | 0.001568 |
| 2458427.865445 | 50.715293 | 0.001790 |
| 2458428.885210 | 50.710343 | 0.001858 |
| 2458429.878247 | 50.705363 | 0.002148 |
| 2458430.868969 | 50.704790 | 0.002139 |
| 2458431.866554 | 50.709192 | 0.001959 |
| 2458432.864695 | 50.711297 | 0.002983 |
| 2458433.863704 | 50.707989 | 0.002242 |
| 2458435.863006 | 50.711920 | 0.003281 |
| 2458436.868322 | 50.710702 | 0.002222 |
| 2458437.863613 | 50.712726 | 0.002427 |
| 2458438.853823 | 50.713394 | 0.001826 |
| 2458439.859369 | 50.717361 | 0.002336 |
| 2458440.862379 | 50.716105 | 0.002080 |
| 2458441.859926 | 50.713725 | 0.002131 |
| 2458442.849080 | 50.710659 | 0.001948 |
| 2458443.844657 | 50.714536 | 0.001898 |
| 2458444.855085 | 50.716400 | 0.003132 |
| 2458447.861223 | 50.714797 | 0.001954 |
| 2458448.876880 | 50.712833 | 0.001649 |
| 2458451.849406 | 50.709969 | 0.001552 |
| 2458452.853554 | 50.712166 | 0.001676 |
| 2458453.852156 | 50.712087 | 0.001650 |
| 2458454.846568 | 50.713921 | 0.002824 |
| 2458455.847264 | 50.715994 | 0.002547 |
| 2458457.857681 | 50.714818 | 0.002072 |
| 2458458.883306 | 50.705553 | 0.002492 |
| 2458459.876520 | 50.709258 | 0.002313 |
| 2458460.876863 | 50.707196 | 0.002084 |
| 2458462.876840 | 50.710386 | 0.001778 |
| 2458463.885966 | 50.706612 | 0.003069 |
| 2458464.872785 | 50.712723 | 0.002452 |
| 2458466.856987 | 50.709175 | 0.001822 |
| 2458467.872219 | 50.709118 | 0.001622 |
| 2458468.875065 | 50.709605 | 0.001846 |

Continued on next page

**Supplementary Table 2 – continued from previous page**

| Time | RV | $\sigma_{RV}$ |
|---|---|---|
| 2458469.876207 | 50.712902 | 0.002060 |
| 2458471.880630 | 50.710095 | 0.002068 |
| 2458472.853329 | 50.713548 | 0.001744 |
| 2458473.865428 | 50.710438 | 0.001740 |
| 2458474.870476 | 50.703559 | 0.001694 |
| 2458475.869932 | 50.709918 | 0.001864 |
| 2458476.870105 | 50.710445 | 0.001912 |
| 2458477.867532 | 50.705179 | 0.002106 |
| 2458478.860757 | 50.704251 | 0.001977 |
| 2458479.857777 | 50.709681 | 0.001770 |
| 2458480.858962 | 50.706970 | 0.002061 |
| 2458481.857194 | 50.710504 | 0.001960 |
| 2458482.857196 | 50.711340 | 0.001755 |
| 2458483.865784 | 50.710626 | 0.002452 |
| 2458484.855122 | 50.713338 | 0.001966 |
| 2458486.871052 | 50.709924 | 0.002876 |
| 2458487.873060 | 50.719476 | 0.002652 |
| 2458488.874811 | 50.717607 | 0.002133 |
| 2458490.869628 | 50.712707 | 0.003140 |
| 2458491.871155 | 50.712421 | 0.003289 |
| 2458500.696528 | 50.710434 | 0.001008 |
| 2458501.868850 | 50.713835 | 0.003843 |
| 2458502.868830 | 50.710266 | 0.002200 |
| 2458503.873334 | 50.717066 | 0.002557 |
| 2458504.871806 | 50.711282 | 0.002841 |
| 2458505.868876 | 50.710407 | 0.002401 |
| 2458506.867784 | 50.715936 | 0.002534 |
| 2458514.819637 | 50.712104 | 0.002212 |
| 2458516.769307 | 50.711504 | 0.002039 |
| 2458517.776056 | 50.714156 | 0.002199 |
| 2458520.690427 | 50.709818 | 0.002070 |
| 2458521.768633 | 50.712338 | 0.003128 |
| 2458522.785743 | 50.713994 | 0.003273 |
| 2458524.784101 | 50.712445 | 0.002141 |
| 2458525.681498 | 50.710051 | 0.002610 |
| 2458528.749016 | 50.707805 | 0.002248 |
| 2458530.798117 | 50.712880 | 0.002710 |
| 2458532.675712 | 50.710372 | 0.001892 |
| 2458535.613838 | 50.712179 | 0.001842 |
| 2458536.654813 | 50.709106 | 0.001915 |

Continued on next page

**Supplementary Table 2 – continued from previous page**

| Time | RV | $\sigma_{RV}$ |
|---|---|---|
| 2458537.738040 | 50.711133 | 0.002107 |
| 2458538.733655 | 50.706642 | 0.002006 |
| 2458539.745830 | 50.708738 | 0.002046 |
| 2458540.746070 | 50.706308 | 0.002298 |
| 2458541.743358 | 50.712370 | 0.001906 |
| 2458542.760933 | 50.711752 | 0.002291 |
| 2458543.748393 | 50.709779 | 0.002020 |
| 2458546.753098 | 50.713940 | 0.002735 |
| 2458547.743954 | 50.710553 | 0.002499 |
| 2458548.734901 | 50.716787 | 0.002673 |
| 2458549.702551 | 50.715159 | 0.002197 |
| 2458550.702951 | 50.711474 | 0.002113 |
| 2458551.691881 | 50.712434 | 0.002475 |
| 2458553.699168 | 50.710700 | 0.003609 |
| 2458554.708289 | 50.712535 | 0.003559 |
| 2458555.695027 | 50.713204 | 0.002506 |
| 2458556.670954 | 50.710185 | 0.002337 |
| 2458557.694168 | 50.708371 | 0.002449 |
| 2458558.680069 | 50.711868 | 0.002365 |
| 2458563.499878 | 50.713783 | 0.001979 |
| 2458564.637856 | 50.712870 | 0.001872 |
| 2458565.625312 | 50.712118 | 0.001902 |
| 2458566.638679 | 50.715963 | 0.002081 |
| 2458567.637140 | 50.714012 | 0.002060 |
| 2458568.635865 | 50.710006 | 0.002271 |
| 2458569.639311 | 50.708798 | 0.001939 |
| 2458570.611197 | 50.712862 | 0.002409 |
| 2458571.639142 | 50.714339 | 0.001990 |
| 2458572.636811 | 50.709935 | 0.003397 |
| 2458591.515118 | 50.708106 | 0.001695 |

Supplementary Table 3: **HARPS-N data.** Nightly-binned radial velocities from the HIRES spectrograph.

| Time [BJD] | RV [m.s$^{-1}$] | $\sigma_{RV}$ [m.s$^{-1}$] |
|---|---|---|
| 2457432.479440 | 50.708009 | 0.002096 |
| 2457433.525206 | 50.710625 | 0.001698 |
| 2457436.466658 | 50.709964 | 0.001559 |
| 2457458.345347 | 50.709066 | 0.001632 |
| 2457460.529560 | 50.715080 | 0.001663 |

Continued on next page

**Supplementary Table 3 – continued from previous page**

| Time | RV | $\sigma_{RV}$ |
|---|---|---|
| 2457461.432945 | 50.713402 | 0.001510 |
| 2457462.497475 | 50.712954 | 0.001784 |
| 2457463.506360 | 50.712423 | 0.001661 |
| 2457502.355499 | 50.708269 | 0.002869 |
| 2457527.369987 | 50.710889 | 0.001979 |
| 2457528.365719 | 50.711293 | 0.002028 |
| 2457529.368742 | 50.709613 | 0.002152 |
| 2457530.378583 | 50.712236 | 0.004212 |
| 2457669.751891 | 50.710147 | 0.001169 |
| 2457670.748257 | 50.711954 | 0.001401 |
| 2457671.744970 | 50.706352 | 0.001272 |
| 2457672.748617 | 50.711848 | 0.001210 |
| 2457673.745447 | 50.713310 | 0.001375 |
| 2457700.763273 | 50.713057 | 0.001482 |
| 2457701.738773 | 50.711171 | 0.001629 |
| 2457702.751730 | 50.707744 | 0.002040 |
| 2457705.755375 | 50.712093 | 0.002079 |
| 2457751.656265 | 50.707807 | 0.003043 |
| 2457753.738897 | 50.712777 | 0.002261 |
| 2457754.702348 | 50.715421 | 0.002113 |
| 2457755.682233 | 50.713446 | 0.001589 |
| 2457756.670723 | 50.711603 | 0.001703 |
| 2457757.617816 | 50.715405 | 0.001271 |
| 2457762.553732 | 50.708360 | 0.002344 |
| 2457763.598677 | 50.712244 | 0.001403 |
| 2457764.541637 | 50.709550 | 0.003013 |
| 2457767.620069 | 50.713187 | 0.002637 |
| 2457769.622253 | 50.710488 | 0.002682 |
| 2457770.535146 | 50.712314 | 0.001608 |
| 2457771.555586 | 50.709511 | 0.001216 |
| 2457772.556130 | 50.707941 | 0.001457 |
| 2457790.610900 | 50.712305 | 0.001296 |
| 2457802.465440 | 50.711858 | 0.001628 |
| 2457803.421712 | 50.707364 | 0.002223 |
| 2457804.454692 | 50.713207 | 0.001833 |
| 2457806.377146 | 50.713499 | 0.002509 |
| 2457807.456705 | 50.708542 | 0.001765 |
| 2457808.543634 | 50.709583 | 0.001529 |
| 2457809.504827 | 50.712031 | 0.002173 |
| 2457810.449306 | 50.709203 | 0.003580 |

Continued on next page

**Supplementary Table 3 – continued from previous page**

| Time | RV | $\sigma_{RV}$ |
|---|---|---|
| 2457814.477335 | 50.715505 | 0.001812 |
| 2457816.413463 | 50.713862 | 0.001811 |
| 2457817.412351 | 50.715299 | 0.003177 |
| 2457823.450914 | 50.714251 | 0.002941 |
| 2457833.395662 | 50.707583 | 0.001870 |
| 2457834.399472 | 50.706090 | 0.002531 |
| 2457835.425559 | 50.715187 | 0.002454 |
| 2457853.485641 | 50.710472 | 0.002170 |
| 2457855.470165 | 50.709825 | 0.002539 |
| 2457856.381144 | 50.713090 | 0.002014 |
| 2457857.380169 | 50.707915 | 0.001598 |
| 2457860.397531 | 50.712403 | 0.001954 |
| 2457861.390190 | 50.710123 | 0.001943 |
| 2457864.447730 | 50.709290 | 0.001994 |
| 2457865.421652 | 50.707580 | 0.001719 |
| 2458098.639134 | 50.708937 | 0.001518 |
| 2458102.569019 | 50.706542 | 0.001797 |
| 2458111.728622 | 50.715540 | 0.001848 |
| 2458119.718817 | 50.717767 | 0.003325 |
| 2458121.644500 | 50.703991 | 0.004328 |
| 2458143.582966 | 50.713350 | 0.003933 |
| 2458144.550619 | 50.720280 | 0.001645 |
| 2458145.461071 | 50.715061 | 0.001824 |
| 2458147.577410 | 50.712937 | 0.001489 |
| 2458184.442259 | 50.709440 | 0.001540 |
| 2458188.596065 | 50.705367 | 0.002775 |
| 2458189.465011 | 50.708191 | 0.002451 |
| 2458190.441182 | 50.713722 | 0.001547 |
| 2458209.430264 | 50.712198 | 0.001247 |
| 2458213.432561 | 50.709860 | 0.001135 |
| 2458214.420090 | 50.709909 | 0.001059 |
| 2458216.417112 | 50.713890 | 0.001393 |
| 2458233.424179 | 50.710543 | 0.001785 |
| 2458234.383031 | 50.709243 | 0.001617 |
| 2458235.419665 | 50.711263 | 0.001592 |
| 2458236.405635 | 50.715474 | 0.001360 |
| 2458242.367787 | 50.713384 | 0.002305 |
| 2458243.369530 | 50.709746 | 0.001984 |
| 2458245.368111 | 50.709252 | 0.002214 |
| 2458246.373651 | 50.709308 | 0.001792 |

Continued on next page

**Supplementary Table 3 – continued from previous page**

| Time | RV | $\sigma_{RV}$ |
|---|---|---|
| 2458248.395437 | 50.705866 | 0.002230 |
| 2458249.393918 | 50.707014 | 0.001755 |
| 2458251.393174 | 50.711522 | 0.003874 |
| 2458252.392918 | 50.713630 | 0.001624 |
| 2458253.397535 | 50.710949 | 0.002564 |
| 2458448.687257 | 50.712610 | 0.001564 |
| 2458449.786381 | 50.705624 | 0.001883 |
| 2458451.759653 | 50.708762 | 0.001741 |
| 2458453.749324 | 50.709194 | 0.001461 |
| 2458454.641412 | 50.708039 | 0.001745 |
| 2458455.726374 | 50.712869 | 0.001883 |
| 2458456.799366 | 50.711768 | 0.003259 |
| 2458473.717630 | 50.708936 | 0.001736 |
| 2458474.669990 | 50.710313 | 0.001459 |
| 2458478.676152 | 50.708418 | 0.001567 |
| 2458479.663565 | 50.713506 | 0.001626 |
| 2458480.718399 | 50.706651 | 0.004291 |
| 2458481.741853 | 50.709593 | 0.001612 |
| 2458482.625993 | 50.711113 | 0.001492 |
| 2458483.627532 | 50.715727 | 0.002028 |
| 2458484.629302 | 50.717120 | 0.001960 |
| 2458486.675026 | 50.705534 | 0.001659 |
| 2458487.674835 | 50.710505 | 0.001776 |
| 2458488.675869 | 50.710522 | 0.002262 |
| 2458489.695305 | 50.716846 | 0.002003 |
| 2458490.541619 | 50.707828 | 0.002220 |
| 2458495.681637 | 50.707658 | 0.001932 |
| 2458502.501660 | 50.717883 | 0.002728 |
| 2458503.577728 | 50.711915 | 0.001388 |
| 2458504.573087 | 50.708935 | 0.002137 |
| 2458506.685884 | 50.709554 | 0.003369 |
| 2458518.592793 | 50.711502 | 0.003535 |
| 2458519.655243 | 50.717455 | 0.004641 |
| 2458520.573851 | 50.710923 | 0.002028 |
| 2458521.591634 | 50.715337 | 0.001524 |
| 2458522.536303 | 50.713643 | 0.001453 |
| 2458523.637970 | 50.709508 | 0.002184 |
| 2458524.497256 | 50.714391 | 0.001384 |
| 2458525.599567 | 50.705518 | 0.003179 |
| 2458526.564357 | 50.705997 | 0.002048 |

Continued on next page

**Supplementary Table 3 – continued from previous page**

| Time | RV | $\sigma_{RV}$ |
|---|---|---|
| 2458527.431427 | 50.709101 | 0.001814 |
| 2458528.400462 | 50.709915 | 0.002181 |
| 2458531.544654 | 50.710336 | 0.002153 |
| 2458536.456395 | 50.707717 | 0.003114 |
| 2458537.529427 | 50.710292 | 0.002297 |
| 2458538.522530 | 50.705452 | 0.002757 |
| 2458539.498388 | 50.707838 | 0.001496 |
| 2458540.578347 | 50.713409 | 0.002213 |
| 2458544.489278 | 50.712052 | 0.001646 |
| 2458545.491144 | 50.708487 | 0.002064 |
| 2458546.433949 | 50.710730 | 0.001981 |
| 2458547.508586 | 50.714460 | 0.001544 |
| 2458548.426992 | 50.708903 | 0.004315 |
| 2458561.434320 | 50.706171 | 0.001847 |
| 2458562.422115 | 50.715680 | 0.003145 |
| 2458563.422789 | 50.715281 | 0.001961 |
| 2458564.429250 | 50.711712 | 0.002393 |
| 2458565.431068 | 50.713467 | 0.001648 |
| 2458566.452271 | 50.713235 | 0.001495 |
| 2458591.420763 | 50.706318 | 0.001511 |
| 2458592.424266 | 50.708173 | 0.002145 |
| 2458593.415883 | 50.704005 | 0.001978 |
| 2458594.417661 | 50.715115 | 0.001773 |
| 2458595.428061 | 50.715062 | 0.001926 |
| 2458596.445636 | 50.708904 | 0.002274 |
| 2458597.416976 | 50.713033 | 0.001883 |
| 2458598.389764 | 50.713729 | 0.001353 |
| 2458604.372132 | 50.706350 | 0.001851 |
| 2458606.371937 | 50.713502 | 0.001601 |
| 2458609.370235 | 50.710477 | 0.001904 |

Supplementary Table 4: **HIRES data.** Nightly-binned radial velocities from the HIRES spectrograph.

| Time [BJD] | RV [m.s$^{-1}$] | $\sigma_{RV}$ [m.s$^{-1}$] |
|---|---|---|
| 2457669.103981 | -0.699 | 0.919 |
| 2457672.121375 | -4.145 | 1.535 |
| 2457673.105029 | -2.949 | 1.360 |
| 2457679.091014 | -0.791 | 1.072 |
| 2457680.130962 | -3.352 | 2.150 |

Continued on next page

**Supplementary Table 4 – continued from previous page**

| Time | RV | $\sigma_{RV}$ |
|---|---|---|
| 2457698.102833 | -0.097 | 1.136 |
| 2457704.051110 | -0.110 | 1.111 |
| 2457715.116001 | -0.067 | 0.999 |
| 2457716.052181 | -5.730 | 1.053 |
| 2457717.035300 | -6.622 | 0.993 |
| 2457718.093415 | -6.147 | 0.775 |
| 2457745.994522 | -0.567 | 1.181 |
| 2457746.980247 | 0.639 | 1.165 |
| 2457747.947147 | -2.009 | 1.125 |
| 2457759.981224 | 7.848 | 1.182 |
| 2457761.880810 | 3.104 | 1.201 |
| 2457763.879316 | 6.863 | 1.161 |
| 2457764.920883 | 3.074 | 1.162 |
| 2457774.879267 | 1.415 | 1.150 |
| 2457775.855511 | -4.948 | 1.186 |
| 2457787.895160 | -5.656 | 1.220 |
| 2457788.837375 | -3.433 | 1.165 |
| 2457789.830950 | -5.309 | 1.287 |
| 2457790.813329 | -2.768 | 1.162 |
| 2457791.804623 | -5.003 | 1.548 |
| 2457802.829787 | 3.807 | 1.152 |
| 2457804.865023 | 0.950 | 1.185 |
| 2457828.839446 | -0.002 | 1.732 |
| 2457829.837713 | 0.783 | 1.152 |
| 2457830.852042 | -2.864 | 1.202 |
| 2457853.826222 | -2.115 | 1.077 |
| 2457854.820125 | -5.645 | 1.212 |
| 2457886.785330 | -3.676 | 1.263 |
| 2458024.121774 | -4.994 | 1.300 |
| 2458029.114341 | -4.135 | 1.084 |
| 2458030.116791 | -7.080 | 1.115 |
| 2458091.936563 | -7.275 | 1.129 |
| 2458098.916938 | -3.805 | 1.168 |
| 2458099.926011 | -1.093 | 1.140 |
| 2458111.903264 | 9.949 | 0.919 |
| 2458112.948622 | 4.599 | 0.800 |
| 2458113.905202 | 4.462 | 0.831 |
| 2458116.900228 | 2.990 | 0.808 |
| 2458117.887758 | 6.150 | 0.936 |
| 2458118.902995 | 4.414 | 0.882 |

Continued on next page

**Supplementary Table 4 – continued from previous page**

| Time | RV | $\sigma_{RV}$ |
|---|---|---|
| 2458124.981199 | 9.315 | 0.857 |
| 2458154.942650 | -8.079 | 2.437 |
| 2458160.961916 | -3.167 | 1.206 |
| 2458181.936113 | 3.981 | 2.310 |
| 2458194.947877 | 7.065 | 1.533 |
| 2458199.787287 | 8.789 | 2.291 |
| 2458386.124139 | -7.261 | 1.145 |
| 2458387.124893 | -7.127 | 1.402 |
| 2458388.116169 | -7.712 | 2.079 |
| 2458389.124517 | -9.835 | 1.445 |
| 2458390.120503 | -4.848 | 1.402 |
| 2458392.115805 | -3.539 | 1.421 |
| 2458393.119747 | -2.629 | 1.256 |
| 2458394.118535 | -3.562 | 1.312 |
| 2458397.108932 | -2.436 | 1.229 |
| 2458427.053677 | 2.624 | 1.188 |
| 2458439.014092 | -6.336 | 3.084 |
| 2458444.042047 | -10.936 | 1.047 |
| 2458476.904461 | -4.766 | 1.439 |
| 2458479.041335 | 3.017 | 1.521 |
| 2458490.969843 | 3.053 | 1.218 |
| 2458491.942657 | 3.596 | 1.101 |
| 2458509.001917 | -2.470 | 1.208 |
| 2458528.922039 | 0.226 | 2.082 |
| 2458568.760850 | -1.659 | 2.127 |
| 2458569.794444 | -0.988 | 2.106 |
| 2458584.767386 | -0.362 | 2.188 |
| 2458595.734981 | 4.804 | 2.100 |
| 2458599.732081 | -2.284 | 2.015 |
| 2458610.755339 | 8.622 | 2.057 |

Supplementary Table 5: **PFS data.** Nightly-binned radial velocities from the PFS spectrograph.

| Time [BJD] | RV [m.s$^{-1}$] | $\sigma_{RV}$ [m.s$^{-1}$] |
|---|---|---|
| 2457449.63819 | 1.09 | 1.71 |
| 2457450.60561 | 1.67 | 1.76 |
| 2457452.60807 | -1.52 | 1.66 |
| 2457468.56635 | -5.27 | 2.09 |
| 2457470.56838 | -3.81 | 2.08 |
| 2457471.57556 | -6.18 | 2.11 |

Continued on next page

**Supplementary Table 5 – continued from previous page**

| Time | RV | $\sigma_{RV}$ |
|---|---|---|
| 2457472.55568 | 0.00 | 2.01 |
| 2457473.58868 | 2.01 | 1.96 |
| 2457474.58707 | -3.33 | 1.96 |
| 2457477.57263 | 3.44 | 2.07 |
| 2457478.56647 | -2.93 | 2.11 |
| 2457498.52942 | -0.58 | 1.72 |
| 2457499.57213 | 8.45 | 2.30 |
| 2457505.55279 | -0.85 | 1.69 |
| 2457507.51060 | -0.48 | 2.37 |
| 2457758.77535 | 5.81 | 1.58 |
| 2457760.72076 | -3.34 | 1.64 |
| 2457762.74949 | -4.45 | 2.38 |
| 2457764.77385 | 3.57 | 2.41 |
| 2457766.83854 | 4.42 | 2.61 |

Supplementary Table 6: **List of parameters used in the preliminary analysis.** The respective priors are provided together with the posteriors.

| Parameter | Prior | Posterior |
|---|---|---|
| *Stellar Parameters* | | |
| Systemic radial velocity $\gamma$ [km.s$^{-1}$] | $\mathcal{U}(49, 51)$ | $50.712 \pm 0.002$ |
| Linear drift $\partial_{RV}$ [m.s$^{-1}$.d$^{-1}$] | $\mathcal{U}(-36.525, 36.525)$ | $0.0 \pm 0.2$ |
| *Planet b Parameters* | | |
| Orbital Period $P_b$ [d] | fixed | $15.5720982$ |
| Transit epoch $T_{0,b}$ [BJD - 2450000] | fixed | $7152.2818$ |
| Radial velocity semi-amplitude $K_b$ [m.s$^{-1}$] | $\mathcal{U}(0, 100)$ | $1.5 \pm 0.2$ |
| Orbital eccentricity $e_b$ | $\mathcal{T}(0.000, 0.083, 0.000, 1.000)$ | $0.05^{+0.06}_{-0.03}$ |
| Argument of periastron $\omega_b$ [°] | $\mathcal{U}(0, 360)$ | $268^{+46}_{-180}$ |
| *Planet c Parameters* | | |
| Orbital Period $P_c$ [d] | fixed | $31.70648$ |
| Transit epoch $T_{0,c}$ [BJD - 2450000] | fixed | $7163.1609$ |
| Radial velocity semi-amplitude $K_c$ [m.s$^{-1}$] | $\mathcal{U}(0, 100)$ | $0.8 \pm 0.2$ |
| Orbital eccentricity $e_c$ | $\mathcal{T}(0.000, 0.083, 0.000, 1.000)$ | $0.05^{+0.06}_{-0.02}$ |
| Argument of periastron $\omega_c$ [°] | $\mathcal{U}(0, 360)$ | $171 \pm 100$ |
| *Planet d Parameters* | | |
| Continued on next page | | |

**Supplementary Table 6 – continued from previous page**

| Parameter | Prior | Posterior |
|---|---|---|
| Orbital Period $P_d$ [d] | $\mathcal{T}(156, 80, 40, 500)$ | $76.2^{+32}_{-0.4}$ |
| Transit epoch $T_{0,d}$ [BJD - 2450000] | fixed | $7166.2604$ |
| Radial velocity semi-amplitude $K_d$ [m.s$^{-1}$] | $\mathcal{U}(0, 100)$ | $0.7 \pm 0.3$ |
| Orbital eccentricity $e_d$ | $\mathcal{T}(0.0, 0.083, 0.0, 1.0)$ | $0.06^{+0.06}_{-0.04}$ |
| Argument of periastron $\omega_d$ [°] | $\mathcal{U}(0, 360)$ | $145^{+150}_{-96}$ |
| *Planet e Parameters* | | |
| Orbital Period $P_e$ [d] | $\mathcal{T}(130, 60, 72, 500)$ | $173^{+2}_{-3}$ |
| Transit epoch $T_{0,e}$ [BJD - 2450000] | fixed | $7142.01954$ |
| Radial velocity semi-amplitude $K_e$ [m.s$^{-1}$] | $\mathcal{U}(0, 100)$ | $0.7 \pm 0.3$ |
| Orbital eccentricity $e_e$ | $\mathcal{T}(0.0, 0.083, 0.0, 1.0)$ | $0.06^{+0.06}_{-0.04}$ |
| Argument of periastron $\omega_e$ [°] | $\mathcal{U}(0, 360)$ | $190 \pm 140$ |
| *Planet f Parameters* | | |
| Orbital Period $P_f$ [d] | $\mathcal{U}(150, 1500)$ | $546 \pm 18$ |
| Transit epoch $T_{0,f}$ [BJD - 2450000] | fixed | $7186.91423$ |
| Radial velocity semi-amplitude $K_f$ [m.s$^{-1}$] | $\mathcal{U}(0, 100)$ | $0.9 \pm 0.2$ |
| Orbital eccentricity $e_f$ | $\mathcal{T}(0.0, 0.083, 0.0, 1.0)$ | $0.06^{+0.06}_{-0.04}$ |
| Argument of periastron $\omega_f$ [°] | $\mathcal{U}(0, 360)$ | $187 \pm 140$ |
| *Planet g Parameters* | | |
| Orbital Period $P_g$ [d] | $\mathcal{N}(62, 1.0)$ | $62.1 \pm 0.3$ |
| Expected transit epoch $T_{0,g}$ [BJD - 2450000] | $\mathcal{U}(7133, 7283)$ | $7152 \pm 5$ |

Continued on next page

**Supplementary Table 6 – continued from previous page**

| Parameter | Prior | Posterior |
|---|---|---|
| Radial velocity semi-amplitude $K_g$ [m.s$^{-1}$] | $\mathcal{U}(0, 100)$ | $1.0 \pm 0.3$ |
| Orbital eccentricity $e_g$ | $\mathcal{T}(0.0, 0.083, 0.0, 1.0)$ | $0.06^{+0.06}_{-0.04}$ |
| Argument of periastron $\omega_g$ [°] | $\mathcal{U}(0.0, 360.0)$ | $154 \pm 120$ |
| *Instrument-related Parameters* | | |
| HARPS jitter $\sigma_{j,\ \mathrm{HARPS}}$ [m.s$^{-1}$] | $\mathcal{U}(0, 100)$ | $2.1 \pm 0.2$ |
| HARPS-N jitter $\sigma_{j,\ \mathrm{HARPS-N}}$ [m.s$^{-1}$] | $\mathcal{U}(0, 100)$ | $2.1 \pm 0.2$ |
| HIRES jitter $\sigma_{j,\ \mathrm{HIRES}}$ [m.s$^{-1}$] | $\mathcal{U}(2, 100)$ | $3.9 \pm 0.4$ |
| PFS jitter $\sigma_{j,\ \mathrm{PFS}}$ [m.s$^{-1}$] | $\mathcal{U}(2, 100)$ | $3.4 \pm 0.9$ |
| HARPS-N offset $\Delta RV_{\mathrm{HARPS-N}}$ [m.s$^{-1}$] | $\mathcal{U}(-1000, 1000)$ | $0.7 \pm 0.3$ |
| HIRES offset $\Delta RV_{\mathrm{HIRES}}$ [km.s$^{-1}$] | $\mathcal{U}(-60.0, 60.0)$ | $50.7124 \pm 0.0005$ |
| PFS offset $\Delta RV_{\mathrm{HARPS-N}}$ [km.s$^{-1}$] | $\mathcal{U}(-60.0, 60.0)$ | $50.713 \pm 0.001$ |

Notes:
- $\mathcal{N}(\mu, \sigma^2)$: Normal distribution with mean $\mu$ and width $\sigma^2$
- $\mathcal{U}(a, b)$: Uniform distribution between $a$ and $b$
- $\mathcal{T}(\mu, \sigma^2, a, b)$: Truncated normal distribution with mean $\mu$ and width $\sigma^2$, between $a$ and $b$

Supplementary Table 7: **List of parameters used in the combined analysis.** The respective priors are provided together with the posteriors.

| Parameter | Prior | Posterior | |
|---|---|---|---|
| | | median and 68.3% C.I. | 95% C.I. |
| *Stellar Parameters* | | | |
| Effective temperature $T_{\rm eff}$ [K] | $\mathcal{N}(6290, 77)$ | $6321^{+48}_{-30}$ | $[6260, 6456]$ |
| Stellar density $\rho_\star/\rho_\odot$ | $\mathcal{N}(0.557, 0.006)$ | $0.563 \pm 0.006$ | $[0.551, 0.573]$ |
| Iron abundance [Fe/H] [dex] | $\mathcal{N}(-0.05, 0.1)$ | $-0.09 \pm 0.07$ | $[-0.23, 0.05]$ |
| Distance to Earth $D$ [pc] | $\mathcal{N}(106.029, 3.353)$ | $103.0^{+1.7}_{-1.3}$ | $[100.3, 106.6]$ |
| Interstellar extinction $E(B-V)$ [mag] | $\mathcal{U}(0, 1)$ | $0.013 \pm 0.01$ | $[0.00, 0.04]$ |
| Systemic radial velocity $\gamma$ [km.s$^{-1}$] | $\mathcal{U}(49, 51)$ | $50.7112 \pm 0.0004$ | $[50.7105, 50.7119]$ |
| Linear limb-darkening coefficient $u_{a,Kp}$ | (derived) | $0.311^{+0.003}_{-0.005}$ | $[0.301, 0.318]$ |
| Quadratic limb-darkening coefficient $u_{b,Kp}$ | (derived) | $0.305^{+0.002}_{-0.001}$ | $[0.302, 0.310]$ |
| Surface gravity log $g$ [cgs] | (derived) | $4.294^{+0.006}_{-0.005}$ | $[4.284, 4.306]$ |
| Stellar luminosity $L_\star/L_\odot$ | (derived) | $1.44^{+0.04}_{-0.02}$ | $[1.40, 1.53]$ |
| Stellar mass $M_\star$ [$M_\odot$] | (derived) | $1.16^{+0.04}_{-0.03}$ | $[1.01, 1.26]$ |
| Stellar radius $R_\star$ [$R_\odot$] | (derived) | $1.27 \pm 0.01$ | $[1.25, 1.30]$ |
| Stellar age $\tau$ [Gyr] | (derived) | $3.1^{+0.4}_{-0.6}$ | $[1.6, 4.0]$ |
| *Planet b Parameters* | | | |
| Orbital Period $P_b$ [d] | $\mathcal{N}(15.572098, 0.0002)$ | $15.57208 \pm 0.00002$ | $[15.57205, 15.57212]$ |
| Transit epoch $T_{0,b}$ [BJD - 2450000] | $\mathcal{N}(7152.2818, 0.012)$ | $7152.283 \pm 0.001$ | $[7152.280, 7152.285]$ |
| Radial velocity semi-amplitude $K_b$ [m.s$^{-1}$] | $\mathcal{U}(0, 100)$ | $1.6 \pm 0.2$ | $[1.2, 2.0]$ |
| Orbital inclination $i_b$ [°] | $\mathcal{S}(82, 90)$ | $88.8 \pm 0.1$ | $[88.5, 89.0]$ |
| Planet-to-star radius ratio $k_b$ | $\mathcal{U}(0.0, 0.1)$ | $0.0187 \pm 0.0002$ | $[0.0183, 0.0191]$ |
| Orbital eccentricity $e_b$ | $\mathcal{T}(0.000, 0.083, 0.000, 1.000)$ | $0.07^{+0.06}_{-0.05}$ | $[0.00, 0.17]$ |

Continued on next page

**Supplementary Table 7 – continued from previous page**

| Parameter | Prior | Posterior | |
|---|---|---|---|
| | | median and 68.3% C.I. | 95% C.I. |
| Argument of periastron $\omega_b$ [°] | $\mathcal{U}(0, 360)$ | $292^{+26}_{-35}$ | $[197, 360]$ |
| System scale $a_b/R_\star$ | (derived) | $21.68 \pm 0.07$ | $[21.52, 21.81]$ |
| Transit impact parameter $b_b$ | (derived) | $0.50^{+0.08}_{-0.07}$ | $[0.39, 0.64]$ |
| Occultation impact parameter $b_{occ,c}$ | (derived) | $0.45^{+0.01}_{-0.03}$ | $[0.39, 0.47]$ |
| Transit duration $T_{14,b}$ [h] | (derived) | $5.15 \pm 0.03$ | $[5.09, 5.20]$ |
| Semi-major axis $a_b$ [AU] | (derived) | $0.128 \pm -0.001$ | $[0.126, 0.132]$ |
| Planet mass $M_b$ [$M_\oplus$] | (derived) | $6.9 \pm 0.9$ | $[5.2, 8.8]$ |
| Planet radius $R_b$ [$R_\oplus$] | (derived) | $2.60^{+0.04}_{-0.03}$ | $[2.53, 2.67]$ |
| Planet bulk density $\rho_b$ [g.cm$^{-3}$] | (derived) | $2.2 \pm 0.3$ | $[1.6, 2.8]$ |
| Planet equilibrium temperature $T_{eq,b}$ [K] | (derived) | $960^{+9}_{-5}$ | $[950, 980]$ |
| *Planet c Parameters* | | | |
| Orbital Period $P_c$ [d] | $\mathcal{N}(31.70648, 0.002)$ | $31.70603 \pm 0.00006$ | $[31.70591, 31.70615]$ |
| Transit epoch $T_{0,c}$ [BJD - 2450000] | $\mathcal{N}(7163.1609, 0.02)$ | $7163.162 \pm 0.002$ | $[7163.158, 7163.166]$ |
| Radial velocity semi-amplitude $K_c$ [m.s$^{-1}$] | $\mathcal{U}(0, 100)$ | $0.8 \pm 0.2$ | $[0.4, 1.2]$ |
| Orbital inclination $i_c$ [°] | $\mathcal{S}(82, 90)$ | $88.48^{+0.04}_{-0.06}$ | $[88.34, 88.61]$ |
| Planet-to-star radius ratio $k_c$ | $\mathcal{U}(0.0, 0.1)$ | $0.0197 \pm 0.0004$ | $[0.0189, 0.0204]$ |
| Orbital eccentricity $e_c$ | $\mathcal{T}(0.000, 0.083, 0.000, 1.000)$ | $0.04^{+0.05}_{-0.03}$ | $[0.00, 0.13]$ |
| Argument of periastron $\omega_c$ [°] | $\mathcal{U}(0, 360)$ | $135^{+134}_{-90}$ | $[0, 360]$ |
| System scale $a_c/R_\star$ | (derived) | $34.8 \pm 0.1$ | $[34.6, 35.0]$ |
| Transit impact parameter $b_c$ | (derived) | $0.914^{+0.007}_{-0.009}$ | $[0.891, 0.933]$ |
| Occultation impact parameter $b_{occ,c}$ | (derived) | $0.92 \pm 0.08$ | $[0.75, 1.10]$ |
| Transit duration $T_{14,c}$ [h] | (derived) | $3.12 \pm 0.05$ | $[3.02, 3.23]$ |
| Semi-major axis $a_c$ [AU] | (derived) | $0.206 \pm 0.002$ | $[0.202, 0.212]$ |
| Planet mass $M_c$ [$M_\oplus$] | (derived) | $4.4 \pm 1.1$ | $[2.3, 6.8]$ |
| Planet radius $R_c$ [$R_\oplus$] | (derived) | $2.73 \pm 0.06$ | $[2.61, 2.86]$ |

Continued on next page

**Supplementary Table 7 – continued from previous page**

| Parameter | Prior | Posterior | |
|---|---|---|---|
| | | median and 68.3% C.I. | 95% C.I. |
| Planet bulk density $\rho_c$ [g.cm$^{-3}$] | (derived) | $1.2 \pm 0.3$ | $[0.6, 1.8]$ |
| Planet equilibrium temperature $T_{eq,c}$ [K] | (derived) | $757^{+7}_{-4}$ | $[750, 773]$ |
| *Planet d Parameters* | | | |
| Orbital Period $P_d$ [d] | $\mathcal{N}(278.3616, 0.09)$ | $278.36180^{+0.0005}_{-0.0004}$ | $[278.3609, 278.3627]$ |
| Transit epoch $T_{0,d}$ [BJD - 2450000] | $\mathcal{N}(7166.2604, 0.02)$ | $7166.261 \pm 0.001$ | $[7166.258, 7166.264]$ |
| Radial velocity semi-amplitude $K_d$ [m.s$^{-1}$] | $\mathcal{U}(0, 100)$ | $0.1^{+0.2}_{-0.1}$ | $[0.0, 0.4]$ |
| Orbital inclination $i_d$ [°] | $\mathcal{S}(85.0, 90.0)$ | $89.80 \pm 0.02$ | $[89.77, 89.85]$ |
| Planet-to-star radius ratio $k_d$ | $\mathcal{U}(0.0, 0.1)$ | $0.0255 \pm 0.0002$ | $[0.0250, 0.0260]$ |
| Orbital eccentricity $e_d$ | $\mathcal{T}(0.0, 0.083, 0.0, 1.0)$ | $0.06^{+0.06}_{-0.04}$ | $[0.00, 0.17]$ |
| Argument of periastron $\omega_d$ [°] | $\mathcal{U}(0, 360)$ | $175^{+92}_{-59}$ | $[0, 360]$ |
| System scale $a_d/R_\star$ | (derived) | $148.2 \pm 0.5$ | $[147.1, 149.1]$ |
| Transit impact parameter $b_d$ | (derived) | $0.52^{+0.05}_{-0.07}$ | $[0.35, 0.65]$ |
| Occultation impact parameter $b_{occ,d}$ | (derived) | $0.51^{+0.01}_{-0.03}$ | $[0.42, 0.54]$ |
| Transit duration $T_{14,d}$ [h] | (derived) | $12.68 \pm 0.06$ | $[12.56, 12.80]$ |
| Semi-major axis $a_d$ [AU] | (derived) | $0.877^{+0.009}_{-0.007}$ | $[0.862, 0.901]$ |
| Planet mass $M_d$ [$M_\oplus$] | (derived) | $1.4^{+1.7}_{-1.0}$ | $[0.0, 4.4]$ |
| Planet radius $R_d$ [$R_\oplus$] | (derived) | $3.54^{+0.05}_{-0.04}$ | $[3.46, 3.65]$ |
| Planet bulk density $\rho_d$ [g.cm$^{-3}$] | (derived) | $0.2^{+0.2}_{-0.1}$ | $[0.0, 0.6]$ |
| Planet equilibrium temperature $T_{eq,d}$ [K] | (derived) | $367^{+3}_{-2}$ | $[363, 375]$ |
| *Planet e Parameters* | | | |
| Orbital Period $P_e$ [d] | $\mathcal{N}(260.0, 60.0)$ | $368.5 \pm 9.5$ | $[354.9, 392.2]$ |
| Transit epoch $T_{0,e}$ [BJD - 2450000] | $\mathcal{N}(7142.01954, 0.00065)$ | $7142.0184 \pm 0.0005$ | $[7142.0174, 7142.0195]$ |

Continued on next page

**Supplementary Table 7 – continued from previous page**

| Parameter | Prior | Posterior | |
|---|---|---|---|
| | | median and 68.3% C.I. | 95% C.I. |
| Radial velocity semi-amplitude $K_e$ [m.s$^{-1}$] | $\mathcal{U}(0, 100)$ | $1.0 \pm 0.4$ | $[0.3, 1.8]$ |
| Orbital inclination $i_e$ [°] | $\mathcal{S}(85.0, 90.0)$ | $89.84^{+0.07}_{-0.03}$ | $[89.80, 90.00]$ |
| Planet-to-star radius ratio $k_e$ | $\mathcal{U}(0.0, 0.1)$ | $0.0354 \pm 0.0007$ | $[0.0345, 0.0363]$ |
| Orbital eccentricity $e_e$ | $\mathcal{T}(0.0, 0.083, 0.0, 1.0)$ | $0.14 \pm 0.09$ | $[0.00, 0.25]$ |
| Argument of periastron $\omega_e$ [°] | $\mathcal{U}(0, 360)$ | $114 \pm 55$ | $[0, 360]$ |
| System scale $a_e/R_\star$ | (derived) | $178.6 \pm 2.9$ | $[173.8, 185.9]$ |
| Transit impact parameter $b_e$ | (derived) | $0.5^{+0.1}_{-0.2}$ | $[0.0, 0.6]$ |
| Occultation impact parameter $b_{occ,e}$ | (derived) | $0.56^{+0.04}_{-0.20}$ | $[0.0, 0.63]$ |
| Transit duration $T_{14,e}$ [h] | (derived) | $13.1 \pm 0.1$ | $[13.0, 13.3]$ |
| Semi-major axis $a_e$ [AU] | (derived) | $1.06 \pm 0.02$ | $[1.03, 1.10]$ |
| Planet mass $M_e$ [$M_\oplus$] | (derived) | $12 \pm 5$ | $[2.6, 22.4]$ |
| Planet radius $R_e$ [$R_\oplus$] | (derived) | $4.92 \pm 0.09$ | $[4.75, 5.12]$ |
| Planet bulk density $\rho_e$ [g.cm$^{-3}$] | (derived) | $0.5 \pm 0.2$ | $[0.1, 0.8]$ |
| Planet equilibrium temperature $T_{eq,e}$ [K] | (derived) | $335 \pm 4$ | $[327, 342]$ |
| *Planet f Parameters* | | | |
| Orbital Period $P_f$ [d] | $\mathcal{N}(542.07973, 0.043)$ | $542.0798 \pm 0.0001$ | $[542.0794, 542.0800]$ |
| Transit epoch $T_{0,f}$ [BJD - 2450000] | $\mathcal{N}(7186.91423, 0.004)$ | $7186.9143^{+0.0005}_{-0.0004}$ | $[7186.9132, 7186.9156]$ |
| Radial velocity semi-amplitude $K_f$ [m.s$^{-1}$] | $\mathcal{U}(0, 100)$ | $0.9 \pm 0.2$ | $[0.5, 1.3]$ |
| Orbital inclination $i_f$ [°] | $\mathcal{S}(82, 90)$ | $89.97 \pm 0.01$ | $[89.96, 90.00]$ |
| Planet-to-star radius ratio $k_f$ | $\mathcal{U}(0.0, 0.2)$ | $0.0663 \pm 0.0001$ | $[0.0661, 0.0665]$ |
| Orbital eccentricity $e_f$ | $\mathcal{T}(0.0, 0.083, 0.0, 1.0)$ | $0.005^{+0.008}_{-0.003}$ | $[0.000, 0.035]$ |
| Argument of periastron $\omega_f$ [°] | $\mathcal{U}(0, 360)$ | $231^{+105}_{-135}$ | $[0, 360]$ |
| System scale $a_f/R_\star$ | (derived) | $231.1^{+0.7}_{-0.8}$ | $[229.5, 232.5]$ |
| Transit impact parameter $b_f$ | (derived) | $0.12^{+0.03}_{-0.05}$ | $[0.00, 0.18]$ |
| Occultation impact parameter $b_{occ,f}$ | (derived) | $0.12^{+0.03}_{-0.05}$ | $[0.00, 0.18]$ |

Continued on next page

**Supplementary Table 7 – continued from previous page**

| Parameter | Prior | Posterior | |
|---|---|---|---|
| | | median and 68.3% C.I. | 95% C.I. |
| Transit duration $T_{14,f}$ [h] | (derived) | $18.99 \pm 0.01$ | $[18.97, 19.01]$ |
| Semi-major axis $a_f$ [AU] | (derived) | $1.37 \pm 0.01$ | $[1.34, 1.40]$ |
| Planet mass $M_f$ $[M_\oplus]$ | (derived) | $12.3 \pm 3.1$ | $[5.9, 18.6]$ |
| Planet radius $R_f$ $[R_\oplus]$ | (derived) | $9.2 \pm 0.1$ | $[9.0, 9.5]$ |
| Planet bulk density $\rho_f$ [g.cm$^{-3}$] | (derived) | $0.09 \pm 0.02$ | $[0.04, 0.13]$ |
| Planet equilibrium temperature $T_{eq,f}$ [K] | (derived) | $294^{+3}_{-1}$ | $[291, 300]$ |
| *Planet g Parameters* | | | |
| Orbital Period $P_g$ [d] | $\mathcal{N}(62, 1.0)$ | $62.1 \pm 0.3$ | $[61.5, 62.7]$ |
| Expected transit epoch $T_{0,g}$ [BJD - 2450000] | $\mathcal{U}(7133, 7283)$ | $7152 \pm 5$ | $[7140, 7160]$ |
| Radial velocity semi-amplitude $K_g$ [m.s$^{-1}$] | $\mathcal{U}(0, 100)$ | $1.0 \pm 0.2$ | $[0.6, 1.5]$ |
| Orbital eccentricity $e_g$ | $\mathcal{T}(0.0, 0.083, 0.0, 1.0)$ | $0.06^{+0.06}_{-0.04}$ | $[0.00, 0.16]$ |
| Argument of periastron $\omega_g$ [°] | $\mathcal{U}(0.0, 360.0)$ | $141^{+60}_{-69}$ | $[0, 360]$ |
| Semi-major axis $a_g$ [AU] | (derived) | $0.323^{+0.004}_{-0.003}$ | $[0.316, 0.331]$ |
| Planet minimum mass $M_g$ $[M_\oplus]$ | (derived) | $7.0^{+1.5}_{-1.4}$ | $[4.1, 9.7]$ |
| Planet equilibrium temperature $T_{eq,g}$ [K] | (derived) | $605^{+6}_{-3}$ | $[599, 618]$ |
| *Instrument-related Parameters* | | | |
| HARPS jitter $\sigma_{j,\ \mathrm{HARPS}}$ [m.s$^{-1}$] | $\mathcal{U}(0, 100)$ | $2.0 \pm 0.2$ | $[1.6, 2.3]$ |
| HARPS-N jitter $\sigma_{j,\ \mathrm{HARPS-N}}$ [m.s$^{-1}$] | $\mathcal{U}(0, 100)$ | $2.1 \pm 0.2$ | $[1.7, 2.6]$ |
| HIRES jitter $\sigma_{j,\ \mathrm{HIRES}}$ [m.s$^{-1}$] | $\mathcal{U}(2, 100)$ | $3.9 \pm 0.4$ | $[3.1, 4.8]$ |
| PFS jitter $\sigma_{j,\ \mathrm{PFS}}$ [m.s$^{-1}$] | $\mathcal{U}(2, 100)$ | $3.5^{+0.9}_{-0.7}$ | $[2.0, 5.2]$ |
| HARPS-N offset $\Delta RV_{\mathrm{HARPS-N}}$ [m.s$^{-1}$] | $\mathcal{U}(-1000, 1000)$ | $0.6 \pm 0.3$ | $[0.0, 1.3]$ |
| HIRES offset $\Delta RV_{\mathrm{HIRES}}$ [km.s$^{-1}$] | $\mathcal{U}(-60.0, 60.0)$ | $50.7122 \pm 0.0005$ | $[50.7111, 50.7132]$ |

Continued on next page

**Supplementary Table 7 – continued from previous page**

| Parameter | Prior | Posterior | |
|---|---|---|---|
| | | median and 68.3% C.I. | 95% C.I. |
| PFS offset $\Delta RV_{\mathrm{HARPS-N}}$ [km.s$^{-1}$] | $\mathcal{U}(-60.0, 60.0)$ | $50.712 \pm 0.001$ | $[50.710, 50.714]$ |
| *K2C5* contamination [%] | $\mathcal{T}(0.0, 0.5, 0.0, 100)$ | $0.2^{+0.2}_{-0.1}$ | $[0.0, 0.6]$ |
| *K2C5* jitter $\sigma_{j,\ K2C5}$ [ppm] | $\mathcal{U}(0.0, 10^5)$ | $12^{+5}_{-6}$ | $[0, 20]$ |
| *K2C5* out-of-transit flux | $\mathcal{U}(0.99, 1.01)$ | $1.000004^{+0.000003}_{-0.000002}$ | $[0.999999, 1.000009]$ |
| *K2C18* contamination [%] | $\mathcal{T}(0.0, 0.5, 0, 100)$ | $0.3^{+0.2}_{-0.2}$ | $[0.0, 0.8]$ |
| *K2C18* jitter $\sigma_{j,\ K2C18}$ [ppm] | $\mathcal{U}(0.0, 10^5)$ | $2^{+2}_{-1}$ | $[0, 6]$ |
| *K2C18* out-of-transit flux | $\mathcal{U}(0.99, 1.01)$ | $0.9999975 \pm 0.000002$ | $[0.999994, 1.000001]$ |
| SED jitter [mag] | $\mathcal{U}(0.0, 0.1)$ | $0.02^{+0.02}_{-0.01}$ | $[0.00, 0.06]$ |

Notes:

C.I. stands for credible interval

• $\mathcal{N}(\mu, \sigma^2)$: Normal distribution with mean $\mu$ and width $\sigma^2$

• $\mathcal{U}(a, b)$: Uniform distribution between $a$ and $b$

• $\mathcal{S}(a, b)$: Sine distribution between $a$ and $b$

• $\mathcal{T}(\mu, \sigma^2, a, b)$: Truncated normal distribution with mean $\mu$ and width $\sigma^2$, between $a$ and $b$
